# Supplementary material for: Set Based Stochastic Subsampling
Source: arXiv:2006.14222 source file (2022-05-30)
Supplement: Supplementary file 1 [file function_appendix.tex]

\begin{figure*}
\centering
\includegraphics[width=1.0\linewidth]{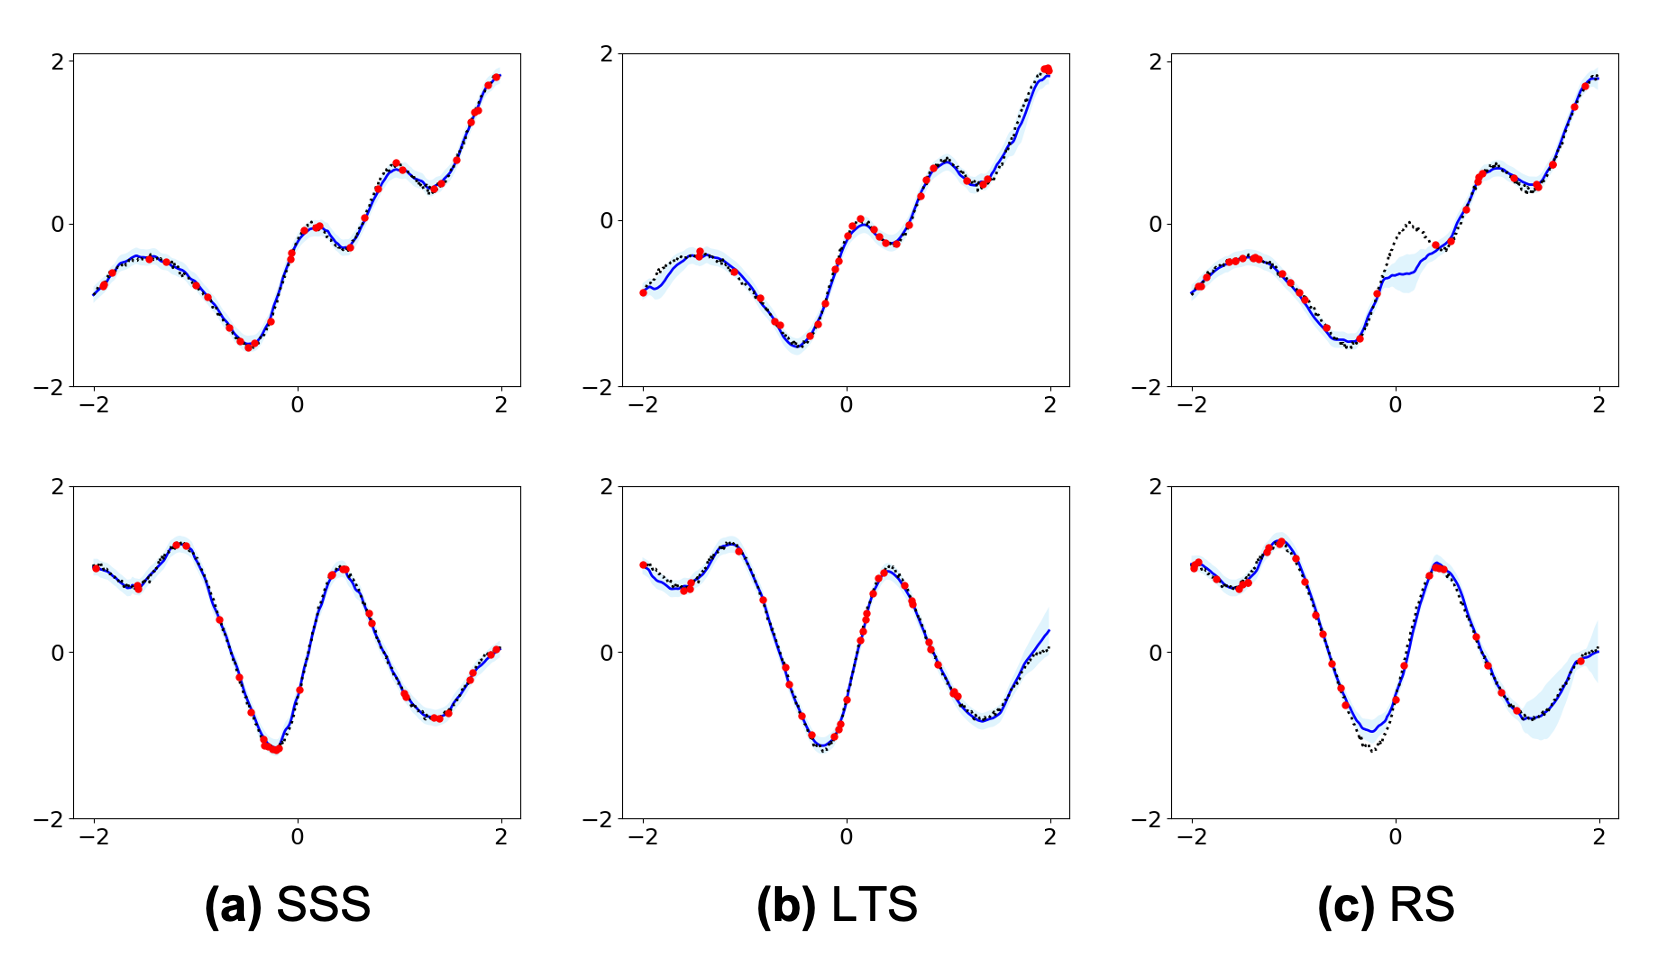}
\caption[Reconstruction samples of 1D functions with different selection methods]{\small Reconstruction samples of 1D functions with different selection methods}
\label{sample_function_appendix}
\end{figure*}
