# Supplementary material for: Set Based Stochastic Subsampling
Source: arXiv:2006.14222 source file (2022-05-30)
Supplement: Supplementary file 2 [file supplementary.tex]

\appendix

\section{Organization}\label{app:organization}

\paragraph{Organization} This supplementary file is organized as follows. We provide the full pseudo-code for the Greedy Training Algorithm and
Fixed-size Subsampling Algorithm and illustrate the generative process of each task using graphical models. We then provide qualitative 
results for the 1D function reconstruction task, qualitative results on the ablation studies and sample visualizations for the CelebA reconstruction
task, Instance Selection and on Instance Selection as applied to few-shot classification on the \textit{mini}ImageNet dataset. Finally we provide 
more details on specifications of models used in the experiments. 

\textbf{Code.} We provide source code at \url{https://github.com/AnonymousRepo2222/SSS}.

\input{algorithms/greedy}

\section{Greedy Training Algorithm} In order to reduce the computational cost at training time, we use a greedy training algorithm with stochastic gradient descent as described in  Algorithm~\ref{greedy-training}. It selects only the top $l$ elements from the candidate set to train the auto-regressive model by minimizing the target loss on the selected samples and randomly selects the remaining $k-l$ elements from the candidate set. As a result, we do not have to run the auto-regressive model  $k/l$ time during training, which significantly reduces the computational cost and shows reasonable performance.

\input{algorithms/fixed_size_sss}
\section{Fixed-size Subsampling}
At test time,  we run the fixed size subsampling algorithm to choose the most task relevant elements from the  set $D$, as described in Algorithm~\ref{fixed-size-selection}. We do not use the greedy training algorithm. Instead, we autoregressively select $k$ elements from the candidate set $D_c$ as described in line 12 from Algorithm~\ref{fixed-size-selection} to construct the representative subset $D_s$. 

\section{Graphical Model}
In Figure~\ref{zm}, we illustrate the generative process using graphical models for each tasks --- (a) feature selection for set reconstruction, (b) feature selection for prediction (c) Instance selection for representative data points and (d) instance selection for few-shot classification. Only the shaded circles denote observable variable and the others are latent variables.

\input{figures/graphical_models}

\section{Instance Selection Samples}
In this section, we show more examples of our 1D and CelebA experiments on how the models select the set elements for the target task.

\subsection{1D Function - Reconstruction}
\input{figures/function_reconstruction_appendix}
Figure~\ref{reconstruction-functions-appendix} shows the reconstruction samples of our model on the 1D function dataset, which is objectively better than that
of Learning to Sample (LTS) or Random Subset (RS). Since RS selects the set elements randomly, it can leave out important part of the 1D curve leading
to wrong reconstructions. LTS also selects insufficient amount of set elements in some parts of the curves, resulting in suboptimal reconstructions. 

\input{figures/celeba_reconstruction_appendix}
\input{figures/celeba_appendix}
\subsection{CelebA}
Figure~\ref{celeba_reconstruction_appendix} shows samples of reconstructed images for varying selection number of pixels. Additionally in 
Figure~\ref{celeba_pixels}, we show the selected pixels of our model for both the classification and reconstruction task. For the attribute
classification task, the model tends to select pixels mainly from the face, since the task is to classify characteristics of the person. For
reconstruction, the selected pixels are more evenly distributed, since the background also contributes significantly to the reconstruction loss.

\section{Dataset Distillation: Instance Selection} 
For the instance selection experiments, we construct a set by randomly sampling 200 face images from the full dataset. To evaluate the model, we
create multiple such datasets and run the baselines(Random Sampling, K-Center Greedy and FPS) and SSS on the same datasets. The FID metric is then computed on the
instances and averaged on all the randomly constructed datasets. For FPS, we use the open-source implementation in
~\href{FPS}{\url{https://github.com/rusty1s/pytorch\_cluster}}. Further, we provide qualitative results on a single dataset in Figure ~\ref{supp_celeba}
where we show how our model picks 5 instances from the full set of 200 images face images.
\input{figures/celeba_instance_appendix}

\subsection{Dataset Distillation: Classification}
In Figure ~\ref{miniImagenet} we provide visualizations for the instance selection problem as applied to the few-shot classification task. Here, we go
from a 20-shot to a 1-shot classification problem where the prototype is selected from the support using SSS. The selected subset is then used in place 
of the support set and used to classify new query instances. 
\input{figures/miniimagenet_appendix}

\section{Model Specifications}\label{appendix:C}
In this section, we describe the main components of our Stochastic Subset Selection models --- $g(d), \rho(\overline{d})$ and $\varphi \circ f(D^{(t)}_c, D_s^{(t-1)})$.

For all the experiments, we use $g$ feedforward neural network with ReLU to project each instance $d$ to lower dimension and average it to encode set representation $D_e$, following DeepSets~\cite{zaheer2017deep}. 

We parameterize $\rho(\cdot)$ with a 3 layered feedforward neural network $h$ followed by sigmoid function as follows as described in Equation (2) from Section 3.3. For $\varphi \circ f$, we use conv-net to extract feature map for each instances in $D^{(t)}_c, D^{(t-1)}_s$ and feed it to set transformer~\cite{lee2018set} for set classification as follows:
\begin{equation}
\begin{gathered}
    f(D^{(t)}_c, D^{(t-1)}_s) = \text{MAB}(D^{(t)}_c, D^{(t-1)}_s) \\
    \text{MAB}(D^{(t)}_c, D^{(t-1)}_s)  = \text{LayerNorm}(H +\text{rFF}(H)) \\
    H=\text{LayerNorm}(D^{(t)}_c + \text{Multihead}(D^{(t)}_c, D^{(t-1)}_s,D^{(t-1)}_s))
\end{gathered}
\end{equation}
where rFF  is a row-wise feedfoward layer which processes each instance independently and Multihead denotes Multihead Attention~\cite{transformer} with each slot of Multihead$(\cdot, \cdot,\cdot)$ representing query, key, and value, respectively.
For the other experiments, we use Deepsets for $f$. We use linear layer for $\varphi$ to output logits for each element in $D_s^{(t-1)}$.

\subsection{Attention}
We details on Attention and Multihead Attention here for completeness. For a more thorough exposition, we refer the reader to 
\citet{transformer} and \citet{lee2018set}.

An attention module computes the following interactions using the dot product:
\begin{equation}
    \text{Att}(Q, K, V; \omega) = \omega (QK^{\top})V
\end{equation}
where $Q \in \mathbb{R}^{n \times d_q}$ are the $n$ query vectors each with of dimension $d_q$. $K \in \mathbb{R}^{n_v \times d_q} \text{ and } 
V \in \mathbb{R}^{n_v \times d_q}$ are the keys and values respectively. Interactions are modelled through $QK^{\top}$ and $\omega$ is an 
activation function such as Softmax or Sigmoid.

Multihead attention projects $Q, K, V$ to $h$ different vectors each with $d_q^M, d_q^M, d_v^M$ dimensions and computes $h$ different 
attention modules according to the following:
\begin{equation}
    \text{Multihead}(Q, K, V; \lambda, \omega) = \text{concat}(O_1, \ldots, O_h)W^{O}
\end{equation}
where
\begin{align}
    O_j &= \text{Att}(QW_j^Q, KW_j^K, VW_j^V; \omega_j)
\end{align}
The Multihead Attention module has learnable parameters $\lambda$ where $\lambda = \{W_j^Q, W_j^K, W_j^V\}_{j=1}^{h}$ and 
$W_j^Q, W_j^K \in \mathbb{R}^{d_q \times d_q^M}$, $W_j^V \in \mathbb{R}^{d_v \times d_v^M}$ and $W^O \in \mathbb{R}^{hd_v^M \times d}$. In all 
our experiments, we use Sigmoid as the activation function.

\section{Function Reconstruction: Ablation}
In the ablation studies in Section 4.4 of the main paper, we investigated the contribution of the Candidate Selection stage (Stage 1) and  the 
AutoRegressive subset selection stage (Stage 2). Additionally, we replaced Stage 1 with random selection in SSS and compare the performance of 
these three variants with SSS. In Figure~\ref{function_reconstruction_ablation}, we provide qualitative results on the function reconstruction 
tasks for these 3 variants as well as SSS. Figure~\ref{function_reconstruction_ablation} is meant to supplement the results presented in 
Section 4.4 of the paper. As can be seen from the figure, using the Candidate Selection stage only to select elements generally focuses on the difficult 
sections of the curves ignoring the other parts which are relatively easier to reconstruct and this results in poorer overall reconstructions. The 
Autoregressive Subset Selection stage on the other hand selects elements that reconstruct the functions well. The downside to this model is that it 
requires a large amount of computation since we have to execute the interactions model for all elements in the input set and this renders this model 
impractical. On the other hand, the model that replaces the Candidate Selection stage in SSS with Random Selection performs better than using only the 
Candidate Selection stage only but results in function reconstruction that a sub-par compared to the Autoregressive Stage only and SSS. This is because 
using random selection in place of the first stage can ignore elements from certain parts of the function when we randomly sample the candidate set 
and hence these parts cannot be reconstructed since the second stage cannot select elements from those regions. This behaviour can be seen in some of
the functions in the second column of Figure~\ref{function_reconstruction_ablation}. In conclusion, SSS offers a good trade-off between computation and
performance and results in better reconstructions since both the Candidate Selection stage and AutoRegressive Subset Selection stages work together
to select the most relevant elements for the task.
\input{figures/function_reconstruction_ablation}
