# Supplementary material for: Set Based Stochastic Subsampling
Source: arXiv:2006.14222 source file (2022-05-30)
Supplement: Supplementary file 3 [file fid_appendix.tex]

\begin{table*}
\begin{center}
\resizebox{\linewidth}{!}{
\begin{tabular}{ccccccc}
    \toprule
    \#Instances       & 2  & 5 & 10 & 15 & 20 & 30   \\
    \midrule
    FPS     &   6.5014 $\pm$ 4.3502 & 4.5098 $\pm$ 2.3809 & 3.0746 $\pm$ 1.0979 & 2.7458 $\pm$ 0.6201 & 2.7118 $\pm$ 1.0410 & 2.2943 $\pm$ 0.8010\\
    Random  &   3.7309 $\pm$ 1.1690 & 1.1575 $\pm$ 0.6532 & 0.8970 $\pm$ 0.4867 & 0.3843 $\pm$ 0.2171 & 0.3877 $\pm$ 0.1906 & 0.1980 $\pm$ 0.1080 \\
    SSS     &   \textbf{2.5307 $\pm$ 1.3583} & \textbf{1.0186 $\pm$ 0.1982} & \textbf{0.5922 $\pm$ 0.3181} & \textbf{0.3331 $\pm$ 0.1169} & \textbf{0.2381 $\pm$ 0.1153} & \textbf{0.1679 $\pm$ 0.0807}\\
    \bottomrule
 \end{tabular}}
  \caption{\small FID Score for varying Instance Selection \label{table:fid_table}}
\end{center}
\end{table*}
